# Supplementary material for: Vocabulary Adaptation for Distant Domain Adaptation in Neural Machine Translation
Source: arXiv:2004.14821 source file (2020-10-31)
Supplement: Supplementary file 1 [file appendix.tex]

\documentclass[11pt,a4paper]{article}
\usepackage[hyperref]{emnlp2020}
\usepackage{times}
\usepackage{latexsym}
\usepackage{amsmath}
\usepackage{amssymb}
\usepackage{bm}

\title{Supplemental Material}
\aclfinalcopy % Uncomment this line for the final submission

\begin{document}
 %\maketitle

\appendix
% \section{Detailed Hyperparameters}
\end{document}
